# Supplementary material for: Bezier Reachable Polytopes: Efficient Certificates for Robust Motion Planning with Layered Architectures
Source: arXiv:2411.13506 source file (2024-11-20)
Supplement: Supplementary file 1 [file Appendix.tex]

\section{Appendix}
\subsection{B\'ezier Curves}
At the cornerstone of the constructive methods discussed in this work is the notion of B\'ezier curves, a polynomial curve which will serve as a useful parameterization for producing kinodynamically admissible trajectories.
A curve $\b b:I\triangleq[0,\time] \to \R^m$ for $\time\in\R_{>0}$ is said to be a B\'ezier curve of order $\order\in\mathbb{N}$ if it is of the form:
\begin{align*}
    \b b(t) = \b z(t)^\top \b \xi,
\end{align*}
where $\b z:I \to \R^{\order+1}$ is a Bernstein basis polynomial of degree $\order$ defined elementwise as:
\begin{align*}
	z_k(t) = \binom{\order}{k} \left(\frac{t}{\time}\right)^k\left(1-\frac{t}{\time}\right)^{\order-k},~~ k=0,\ldots,\order,
\end{align*}
and $\b \xi \in \R^{\order+1\times m}$ are a collection of $\order+1$ \textit{control points}. Defining a phasing variable over the interval $I$ as $\tau:t\mapsto\frac{t}{\time}$, B\'ezier curves can be rewritten in matrix form as follows:
\begin{align*}
	\b b(t) = \underbrace{\begin{bmatrix}1&\tau(t)&\cdots&\tau^p(t)\end{bmatrix}}_{\b T(t)}\underbrace{\b P \b L^{-1}}_{\b M} \b \xi,
\end{align*}
where $\b T:I\to \R^{p+1}$ parameterizes time, $\b P\in\R^{p+1\times p+1}$ is a diagonal matrix with entries equal to the binomial expansion of dimension $p+1$ and $\b L\in \R^{p+1\times p+1}$ is the lower triangular Pascal matrix \cite{https://web.mit.edu/18.06/www/Essays/pascal-work.pdf}.

Differentiating a B\'ezier curve of order $\order$ results in a B\'ezier curve of order $p-1$ defined via:
\begin{align*} 
    \dot{\b b}(t) = \b z(t)^\top \b S_\time \b \xi
\end{align*}
where the matrix $\mb S_\time \in \mathbb{R}^{p\times p+1}$ as:
\begin{align*}
    \mb S_{\time,ii} &= -\frac{p}{\time}, ~~\mb S_{\time,i,i+1}(\time) = \frac{p}{\time},~~i=1,\ldots,p,
\end{align*}
with zeros everywhere else.
Given a B\'ezier curve of order $\order$, we can raise it to a curve of order $\order+1$ with control points $\b R^p\b \xi$ where $\mb R^p \in \mathbb{R}^{p+1\times p}$ contains all zeros except:
\begin{align*}
    \mb R^p_{ii} &= \frac{p+1-i}{p}, ~~ \mb R^p_{i+1,i} = \frac{i}{p},~~i=1,\ldots,p.
\end{align*}
The matrix $\b R$ is taking a convex combination of the existing control points by evaluating the Bernstein basis polynomials at intermediate points along the curve. 
The process of curve refinement can be iterated to refine a curve arbitrarily to order $o>p$ with control points $\b R^o\cdots \b R^{p+1}\b R^p \b\Xi$. 

With these tools, we can construct a matrix $\b H\in\R^{p+1\times p+1}$ relating a B\'ezier curve to its derivatives via a B\'ezier curve of the same order as $\b b$ defined as:
\begin{align*}
    \dot {\b b}(t) = \b z(t)^\top \underbrace{\b R^p\b S_\tau}_{\b H} \b \xi
\end{align*}

Next, we introduce the notion of B-splines as a piecewise continuous collection of B\'ezier curves. A $j-$segmented B-spline of order $p$ is simply a collection of order $p$ B\'ezier curves connected with $C^0$ continuity. We can split an order $p$ Be\'zier curve into a $k$ segmented B-spline of order $p$ for any $k\in\mathbb{N}$. This is accomplished via a matrix $\b Q_i$, $i=1,\ldots,k$, defined as:
\begingroup
	
	\setlength{\arraycolsep}{2pt}
\begin{align*}
	\sigma_i &\triangleq \begin{cases}\frac{k-i}{k-i+1}&i<k\\1&i=k\end{cases}\\
		\b Z(\sigma_i) &\triangleq \begin{bmatrix}1&&&\\&\sigma_i&&\\&&\ddots&\\&&&\sigma_i^p\end{bmatrix},~\b Z'(\sigma_i) \triangleq \begin{bmatrix}1&&&\\&(1-\sigma_i)&&\\&&\ddots&\\&&&(1-\sigma_i)^p\end{bmatrix}\\
		\b Q^u_i &\triangleq \b M^{-1} \b Z(\sigma_i) \b M,\\
	\b Q^l_i &\triangleq \begin{bmatrix}\b 0 &&1 \\ &\rddots&\\1&&\b 0\end{bmatrix}\b M^{-1}\b Z'(\sigma_i) \b M \begin{bmatrix}\b 0 &&1 \\ &\rddots&\\1&&\b 0\end{bmatrix}\\ 
 \b Q_i &\triangleq \b Q^u_i \b Q^l_{i-1} \cdots \b Q^l_{0},
 \end{align*}
\endgroup
This notion will be useful when comparing B\'ezier curves with reference B-splines.

\subsection{Vectorization}
In this section, we will review matrix vectorization, its properties, and will explicitly define the vectorized matrices discussed in the text. Cosider matices $\b A\in\R^{n\times m}$ and $\b B\in\R^{k\times l}$. The vectorized versions of these matrices $\b a\triangleq\text{vec}(\b A)\in\R^{nm}$ and $\b b\trianlgeq\text{vec}(\b B)\in\R^{kl}$ are defined as:
\begin{align*}
	\b a_{i+nj} &= \b A_{i,j},~~i=0,\ldots,n,~~j=0,\ldots m\\
	\b b_{i+lj} &= \b B_{i,j},~~i=0,\ldots,k,~~j=0,\ldots l
\end{align*}
i.e., they take the columns of the matrices and stack them vertically. There are a number of useful properties related to vectorization, summarized here:
\begin{align*}
	\b a &= \b K^{(n,m)} \text{vec}(\b A^\top) \\
	\text{vec}(\b A \b B) &= (\b I_l \otimes \b A)\text{vec}(\b B) = (\b B^\top \otimes \b I_n)\text{vec}(\b A)
\end{align*}
where $\b K^{(n,m)}\in\R^{mn\times nm}$ is the commutation matrix, and $\otimes$ is the Kronecker product.

Using these properties, we can transform \red{equation (14)} into $\b \xi = \b H_{\text{vec}}\bez$ via:
\begin{align*}
	\b \xi &= \text{vec}(\b\Xi) = \text{vec}\left(\begin{bmatrix}\Bez\b H^0 \\\vdots\\\Bez\b H^{\gamma-1}\end{bmatrix}\right)\\
	&= (\b K^{(p+1,\gamma)}\otimes \b I_m)\begin{bmatrix}\text{vec}(\Bez\b H^0) \\\vdots\\\text{vec}(\Bez\b H^{\gamma-1})\end{bmatrix}\\
\end{align*}
	&=(\b K^{(p+1,\gamma)}\otimes \b I_m)\begin{bmatrix}(\b H^{0\top}\otimes \b I_m)\bez \\\vdots\\(\b H^{\gamma-1\top}\otimes \b I_m)\bez\end{bmatrix}\\
		&=\underbrace{(\b K^{(p+1,\gamma)}\otimes \b I_m)\begin{bmatrix}(\b H^{0\top}\otimes \b I_m) \\\vdots\\(\b H^{\gamma-1\top}\otimes \b I_m)\end{bmatrix}}_{\b H_{\text{vec}}}\bez
\end{align*}

Next, we can consider \red{equation (15)} as:
\begin{align*}
	\text{vec}(\b\Xi\b\Delta) &= \text{vec}(\begin{bmatrix}\b x_d(0) & \b x_d(\time)\end{bmatrix})\\
		\underbrace{(\b \Delta^\top \otimes \b I_n)}_{\triangleq \b \Delta_{\text{vec}}}\b\xi &= \begin{bmatrix}\b x_d(0) \\ \b x_d(\time)\end{bmatrix}
\end{align*}
whereby we can reformulate this to a constraint on $\bez$ via:
\begin{align*}
	\underbrace{\b\Delta_{\text{vec}}\b H_{\text{vec}}}_{\b D_{\text{vec}}} \bez = \begin{bmatrix}\b x_d(0) \\ \b x_d(\time)\end{bmatrix}
\end{align*}
